# Supplementary material for: Field-induced negative differential spin lifetime in silicon
Source: arXiv:1108.4907 source file (2011-09-30)
Supplement: Supplementary file 1 [file supp_aux.pdf]

# Supplemental material to the paper “Field-induced negative differential spin lifetime in silicon”

Jing Li,<sup>1</sup> Lan Qing,<sup>2</sup> Hanan Dery,<sup>2,3</sup> and Ian Appelbaum<sup>1,\*</sup>

<sup>1</sup>*Department of Physics and Center for Nanophysics and Advanced Materials,  
University of Maryland, College Park, Maryland 20742*

<sup>2</sup>*Department of Physics and Astronomy, University of Rochester, Rochester, New York 14627*

<sup>3</sup>*Department of Electrical and Computer Engineering, University of Rochester, Rochester, NY 14627*

**1. Experimental device.** In our all-electrical devices (schematic band diagram shown in Fig. I), spin-polarized hot electrons are injected from a ferromagnetic tunnel-junction cathode and travel ballistically across a nonmagnetic thin-film anode and over a rectifying Schottky barrier, into the conduction band of undoped Si(100) with their spin axis in the device plane [S1]. This 225-micron-thick crystalline Si channel wafer was float-zone grown and has a room-temperature resistivity of 4 k $\Omega$ ·cm due to unintentional doping. The spin signal due to transport of this current ( $I_{C1} \approx 30 \mu\text{A}$ ) across  $L = 225 \mu\text{m}$  is measured via spin-dependent inelastic scattering asymmetry through a ferromagnetic thin film. Subsequent collection of the remaining ballistic current component in a second hot-electron collector comprises

the spin signal current  $I_{C2}$  [S2]. The (constant) tunnel-junction injector power is approximately 30 mW, so the change in Joule dissipation in the transport channel due to variation in applied voltage ( $V_{C1}$ ) is only a few percent of this value and unable to account for the depolarization effects we see.

## 2. Monte Carlo simulation.

(a) Band Structure. In each of the six valleys of silicon, we consider ellipsoidal constant energy surfaces as  $\epsilon(\mathbf{k}) = \hbar^2(k_l^2/m_l + k_t^2/m_t)/2$ , where  $l(t)$  denotes the longitudinal (transverse) components.  $m_l = 0.916m_0$ ,  $m_t = 0.191m_0$ . We introduce the Herring-Vogt transformation defined by  $k_i^* = \mathcal{T}_{ij}^n k_j^n$  [S3, S4]. In the  $n^{\text{th}}$  valley frame of reference (centered at the bottom of the valley with the  $z$  axis along its symmetry axis), we take the transformation matrix

$$\mathcal{T}^n = \text{diag}\left(\sqrt{\frac{m_0}{m_t}}, \sqrt{\frac{m_0}{m_t}}, \sqrt{\frac{m_0}{m_l}}\right),$$

and the ellipsoidal constant energy surfaces become spheres. To preserve vector equations,  $\mathcal{T}^n$  is also applied to other vector quantities such as phonon wave vectors.

(b) Initial State. The steady-state distribution at the end of the Monte Carlo simulation is independent of the initial distribution. Therefore, we choose simple Maxwellian distributions as initial condition in each valley (product of three independent zero-mean Gaussians of  $k_x^*$ ,  $k_y^*$ ,  $k_z^*$  with  $m_0 k_B T / \hbar^2$  as the variance).

(c) Free Flight. We consider electrons as classical particles accelerated by the electric field  $\mathbf{E}$  when no scattering events happen, i.e.,  $\hbar \mathbf{k}' - \hbar \mathbf{k} = -e \mathbf{E} t$ , where  $t$  is the elapsed time during which the electron's wavevector evolves from  $\mathbf{k}$  into  $\mathbf{k}'$ . Since  $\mathbf{E}$  is parallel to one of the crystallographic axes, the different effective mass components in the field direction leads to different energy accumulations in different valleys, and eventually to the difference between hot and cold valleys.

(d) Rees Self-Scattering. To determine the occurrence of scattering events without the difficulty of solving integral equations for each event, we use the self-scattering technique [S4–S6]. Scattering times are randomized according to a homogeneous Poisson process,  $\propto \exp(-\Gamma_0 t)$ , in which a fictitious self-scattering is included such that the total scattering rate together with the self-scattering is  $\Gamma_0$ . If an electron undergoes a ‘self-scattering’ event,

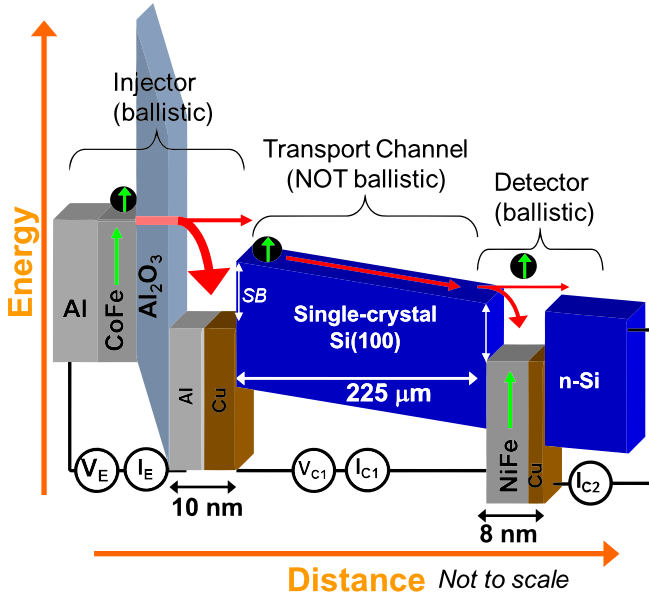

FIG. I: Schematic band diagram of our nonequilibrium spin-polarized electron transport device using a ferromagnetic tunnel junction for hot electron generation of injected current  $I_{C1}$  into the insulating, nominally undoped (room temperature resistivity 4 k $\Omega$ ·cm) Si(100) transport channel. Spin polarization after transport is measured in low magnetic field  $\approx 20$  gauss by the relative difference in the spin signal current  $I_{C2}$  upon changing the detector ferromagnetic magnetization axis, which is due to mean-free-path asymmetry (see Ref. [S2]).

TABLE 1: Integration limits in Eq. (II).

| Condition                                            | Absorption                                                                 | Emission                                         |
|------------------------------------------------------|----------------------------------------------------------------------------|--------------------------------------------------|
| $\epsilon \leq \epsilon_s$ ( $x_\epsilon \leq x_0$ ) | $x_1 = x_0 - \sqrt{x_0 x_\epsilon}$<br>$x_2 = x_0 + \sqrt{x_0 x_\epsilon}$ | absent                                           |
| $\epsilon > \epsilon_s$ ( $x_\epsilon > x_0$ )       | $x_1 = 0$<br>$x_2 = \sqrt{x_0 x_\epsilon} + x_0$                           | $x_1 = 0$<br>$x_2 = \sqrt{x_0 x_\epsilon} - x_0$ |

its wavevector immediately before and after the scattering is unchanged. This technique is valid if  $\Gamma_0$  exceeds the total scattering rate of an electron in state  $\mathbf{k}$ . In the simulation, we use  $\Gamma_0 = 10^{14} \text{ s}^{-1}$ .

(e) Intravalley Acoustic Scattering. We assume the phonon populations inside the crystal not to be disturbed by the electric field. For phonon-assisted transitions, selection rules only allow the acoustic intravalley scattering. We also take the long wavelength approximation without distinguishing between longitudinal and transverse phonons [S7]. With the dimensionless variable:

$$x = \frac{\hbar q v_s}{k_B T} \approx \frac{\hbar q^* v_s}{k_B T} \sqrt{\frac{m_d}{m_0}}, \quad (\text{I})$$

where  $\mathbf{q} = \mathbf{k} - \mathbf{k}'$ , the total scattering rate follows

$$\Gamma_{ac} = \frac{(2m_d)^{\frac{1}{2}}}{\pi} \frac{\Xi^2 (k_B T)^3}{8\hbar^4 \rho v_s^4} \frac{1}{\sqrt{\epsilon}} \int_{x_1}^{x_2} \left( \frac{n_{\mathbf{q}}}{n_{\mathbf{q}+1}} \right) x^2 dx. \quad (\text{II})$$

Here and in Eq. (III) the top (bottom) line refers to absorption (emission).  $m_d = \sqrt[3]{m_l m_t^2}$  is the density-of-state effective mass.  $\Xi = 9.0 \text{ eV}$ ,  $\rho = 2.33 \text{ g/cm}^3$  and  $v_s = 9.04 \times 10^5 \text{ cm/s}$  denote the deformation potential, crystal density and sound velocity, respectively. The integration limits  $x_1$  and  $x_2$  in Eq. (II) are given in Table 1 where  $\epsilon_s = m_d v_s^2/2$ ,  $x_\epsilon = 4\epsilon/k_B T$ ,  $x_0 = 4\epsilon_s/k_B T$ . With the truncated Laurent expansion of phonon distribution:

$$n_{\mathbf{q}}(x) = \begin{cases} 1/x - \frac{1}{2} + \frac{1}{12}x - \frac{1}{720}x^3, & \text{if } x < 3.5, \\ 0, & \text{if } x \geq 3.5, \end{cases}$$

the integration in Eq. (II) can then be performed very easily. For the state after scattering, we choose  $x$  according to the expression inside the integration in Eq. (II) with the rejection technique [S4]. Then  $q^*$  is calculated from Eq. (I), and the angle between  $\mathbf{k}'^*$  and  $\mathbf{k}^*$  is obtained by energy and momentum conservation. The angle of rotation around  $\mathbf{k}^*$  is completely random.

(f) Intervalley Phonon Scattering. Similarly, the selection rules determine the dominant coupling constants for  $f$ -process with LA and TO phonons, and  $g$ -process with LO phonons. The total scattering rate reads [S7]

$$\Gamma_{iv,i} = \frac{(2m_d)^{\frac{3}{2}}}{\pi} \frac{D_{m,i}^2 Z_i}{4\hbar^2 \rho \Omega_{m,i}} \left( \frac{n_{\mathbf{q},i} \sqrt{\epsilon + \Omega_{m,i}}}{(n_{\mathbf{q},i} + 1) \sqrt{\epsilon - \Omega_{m,i}}} \right). \quad (\text{III})$$

TABLE 2: Coupling constants and phonon energies for intervalley  $f$ -process and  $g$ -process scattering.

| Process Mode                | $f$  |      |      | $g$  |      |      |
|-----------------------------|------|------|------|------|------|------|
|                             | TA   | LA   | TO   | TA   | LA   | LO   |
| $i$                         | 1    | 2    | 3    | 4    | 5    | 6    |
| $D_{m,i} [\text{eV/\AA}]$   | 0.15 | 3.4  | 4.0  | 0.50 | 0.80 | 3.0  |
| $\Omega_{m,i} [\text{meV}]$ | 18.1 | 43.1 | 54.3 | 12.1 | 18.1 | 60.3 |

The coupling constant  $D_{m,i}$  and the phonon energy  $\Omega_{m,i}$  of the considered  $i$ th mechanism are listed in Table 2.  $Z_i = 4$  for  $f$ -process and  $Z_i = 1$  for  $g$ -process are numbers of possible final valleys. The final valley for  $f$ -process is chosen randomly. The states after scattering are equally probable on the constant energy surface with energy conservation.

(g) Ionized Impurity Scattering. Using the Brooks-Herring approach [S4], we get a total scattering rate

$$\Gamma_I = \frac{(2m_d)^{\frac{3}{2}}}{\pi} \frac{e^4 N_I}{2\epsilon_0^2 \kappa_S^2 \hbar^4 \beta^4} \sqrt{\epsilon} \left( 1 + \frac{8m_d \epsilon}{\hbar^2 \beta^2} \right)^{-1}, \quad (\text{IV})$$

where  $\kappa_S = 11.7$  is the relative dielectric constant, and we assume  $N_I = 10^{12} \text{ cm}^{-3}$  as the impurity concentration. The screening length  $\beta^{-1}$  is taken as half the average distance  $d = N_I^{-1/3}$  between impurities. With a random number  $r \in (0, 1)$  we generate the scattering angle  $\gamma$  as

$$\cos \gamma = 1 - 2(1-r) \left( 1 + \frac{8m_d \epsilon r}{\hbar^2 \beta^2} \right)^{-1}.$$

The simulation of all the above processes ends after  $\sim 1 \text{ ns}$  when the steady-state distribution is definitely reached. Since such a time is negligible compared to the transit time across  $225 \mu\text{m}$ , the distribution in the entire transport channel can be considered as a steady-state distribution. Physical quantities are simply the averages of  $N \gg 1$  electrons. We repeat the procedure for  $N = 10^6$  particles with various setups of  $T$  and  $\mathbf{E}$ .

**3. Simulated results.** The typical steady-state  $k$ -space distribution in hot or cold valley is shown in Fig. II. Also obtained is the repopulation ratio  $n_c/n_h$  with different setups shown in Fig. 4(b) of the main paper. The drift velocity is obtained by taking the average  $\mathcal{T}^n \mathbf{k}^* \cdot \hat{\mathbf{E}}^*$  times  $\hbar/m_0$ , and the mean energy by the average  $k^{*2}$  times  $\hbar^2/(2m_0)$ . The results are shown in Fig. 3(a)-(b) of the main paper.

The simulated distribution is well approximated by a drifted and heated Maxwellian [S8]:  $f(\mathbf{k}) \sim \exp[-(\hbar \mathbf{k}^* - m_0 \mathbf{v}_d)^2 / 2m_0 k_B T_e]$ . Since the drift velocity,  $v_d$ , is small compared to the average carrier speed, we simply consider a heated Maxwellian ( $v_d \rightarrow 0$ ) and study the distribution as a function of energy as shown in Fig. 4(a) of the main paper. We notice two effective temperatures in

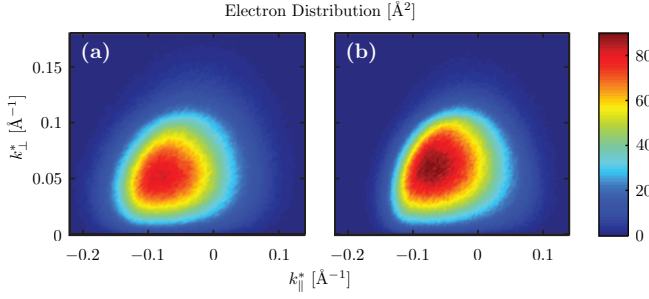

FIG. II: Typical  $k$ -space distributions for electrons in (a) hot and (b) cold valleys at  $T = 60$  K with  $E = 4$  kV/cm.  $k_{\parallel}^*$  ( $k_{\perp}^*$ ) denotes the wave-vector component parallel (perpendicular) to the field  $\mathbf{E}$  after the Herring-Vogt transformation.

either a hot or a cold valley. The sharper decay at the high-energy tail of the distribution is caused by intervalley process scattering which introduces extra cooling for energetic electrons. The effective temperature of the simulated distribution drops around the corresponding phonon energy of  $f$ -process (43.1 meV as in Table 2). Though these hot electrons have a small effect on charge transport, they contribute significantly in spin relaxation (explained in Sec. 4 below).

The spin lifetime with distribution  $f(\mathbf{k})$  reads [S9]

$$\frac{1}{\tau_{s,\nu}} = \frac{2\pi\hbar}{\rho D} \int d^3\mathbf{k} \frac{\partial f(\mathbf{k})}{\partial \epsilon(\mathbf{k})} \int \frac{d^3\mathbf{k}'}{(2\pi)^3} |M_{\nu}^{sf}(\mathbf{k}, \mathbf{k}')|^2 \frac{1}{\Omega_{\nu}(\mathbf{q})} \times \left[ \sum_{\pm} (n_{\nu,\mathbf{q}} + \frac{1}{2} \pm \frac{1}{2}) \delta(\epsilon(\mathbf{k}') - \epsilon(\mathbf{k}) \pm \Omega_{\nu}(\mathbf{q})) \right], \quad (\text{V})$$

where  $D = \int [\partial f(\mathbf{k}) / \partial E_{\mathbf{k}}] d^3\mathbf{k}$  normalizes the integration and  $\nu$  denotes the phonon mode. The  $+$  ( $-$ ) refers to phonon emission (absorption) processes.  $M_{\nu}^{sf}(\mathbf{k}, \mathbf{k}')$  is the spin-flip matrix element between electronic states in the lower conduction band. Table 3 shows the expressions for various spin relaxation processes [S10], where  $\eta \approx 14$  meV $\cdot\text{\AA}$  and  $\Delta'_x \approx 5.0$  meV are spin-orbit coupling parameters.  $\Delta_C \approx 0.5$  eV is the energy spacing between the lower and upper conduction bands at the valley center.  $E_{g,x} \approx 4.3$  eV is the energy gap between the conduction and valence bands at the  $X$  point.  $\kappa \equiv k_x + ik_y$  in the  $z$  valley collinear with the spin-quantization axis, and  $\kappa \equiv k_y$  ( $\kappa \equiv ik_x$ ) in the  $x$  ( $y$ ) valley.  $D_g \approx 4$  eV/ $\text{\AA}$  is a scattering constant in the  $g$ -process associated with a phonon energy of  $\Omega_g \approx 21$  meV.  $D_1 \approx 12$  eV/ $\text{\AA}$  ( $D_3 \approx 5$  eV/ $\text{\AA}$ ) is associated with a phonon mode of  $\Sigma_{1(3)}$  symmetry in the  $f$ -process governed by the upper (middle) acoustic branch with  $\Omega_{f,1} \approx 47$  meV ( $\Omega_{f,3} \approx 23$  meV). We keep the long wavelength approximation  $\Omega_i(\mathbf{q}) = \hbar v_s q$  for intervalley scattering. From the steady-state distribution  $f(\mathbf{k})$  obtained by the simulation, we can perform numerical integrations of Eq. (V) and calculate the total spin relaxation rate  $1/\tau_s$ . The results dependent on  $T$  and  $\mathbf{E}$  are displayed in Fig. 3(c) of the main paper.

TABLE 3: Spin-flip matrix element for different process.

| Process                                   | Intravalley                                     | $f$ -process                        | $g$ -process                                  |
|-------------------------------------------|-------------------------------------------------|-------------------------------------|-----------------------------------------------|
| $ M_{\nu}^{sf}(\mathbf{k}, \mathbf{k}') $ | $\frac{\eta \kappa - \kappa' }{\Delta_C} q \Xi$ | $C_i D_i \frac{\Delta'_x}{E_{g,x}}$ | $\frac{\eta \kappa + \kappa' }{\Delta_C} D_g$ |

The polarization after transport across 225  $\mu\text{m}$  can be calculated as  $\mathcal{P}_0 \exp(-\tau_{tr}/\tau_s)$ , where the mean transit time  $\tau_{tr} = L/v_d$  is calculated from the drift velocity and we assume  $\mathcal{P}_0 \approx 1/8$ . Thus in the main paper, the  $v_d$  and  $\tau_s$  given by Fig. 3(a) & (c) directly lead to the polarization in Fig. 3(d).

**4. Analytical expressions.** The spin-independent transport has been thoroughly studied by solving the Boltzmann transport equation [S8, S11–S13]. A realistic theory has been established by the method of nonequilibrium statistical operators [S14], where analytical balance equations are derived, and accurate  $v_d$  and  $T_{e,\mu}$  can be obtained as the numerical solutions of six transcendental equations. Alternatively, one can use the empirical expressions of  $v_d$  and  $T_e$  (see, e.g., Ref. [S15, S16]).

To derive an analytical expression of the spin relaxation time we start from an elaborate analytical distribution which solves the Boltzmann transport equation with intervalley scattering [S13]. Since this elaborate distribution is close to a heated Maxwellian,  $f(\epsilon) \sim \exp(-\epsilon/k_B T_e)$ , we use the approximation

$$T_e' \approx T + \gamma(T_e - T), \quad (\text{VI})$$

where  $T$  is the lattice temperature, and  $T_e$  is the equivalent temperature from the mean electron energy  $\frac{3}{2}k_B T_e$ . The  $\gamma$  parameter corresponds to the aforementioned cooling effect at the high-energy tail of the distribution due to intervalley processes (relevant energy region for spin relaxation),

$$\gamma \approx 1 - Z \left( \frac{\overline{D}_f}{D_0} \right)^2 \frac{k_B \overline{T}}{\Omega_f} \approx 0.9, \quad (\text{VII})$$

where we take  $\overline{D}_f \approx D_{m,2} \approx 3.4$  eV/ $\text{\AA}$  and  $\overline{\Omega}_f \approx \Omega_{m,2} \approx 43.1$  meV, as given in Table 2, for the dominant  $Z = 4$   $f$ -process.  $D_0 \approx 9.35$  eV/ $\text{\AA}$  is the deformation potential constant for optical phonon scattering [S17]. The average temperature of the experiments is  $\overline{T} \approx 75$  K.

Substituting the heated Maxwellian in conjunction with the  $f$ -processes matrix element of Table 3 into Eq. (V), we derive the spin relaxation time of hot electrons:

$$\frac{1}{\tau_s} \approx \mathcal{C}' \sum_{i=1,3}^{\mu=h,c} \frac{A_{i,\mu} n_{\mu} D_i^2}{\sqrt{\Omega_i}} \frac{\exp(y_i - y'_{i,\mu}) + 1}{\exp(y_i) - 1} F(y'_{i,\mu}), \quad (\text{VIII})$$

where  $A'_{1,h} = 8$  (12),  $A'_{3,h} = 6$  (5),  $A'_{1,c} = 8$  (4) and  $A'_{3,c} = 2$  (3) if the electric field is collinear with (perpendicular to) the spin-quantization axis. The coefficient

$$C' = \frac{2}{\hbar^2 \varrho} \left( \frac{\Delta'_x}{E_{g,x}} \right)^2 \left( \frac{2m_d}{\pi} \right)^{\frac{3}{2}} \approx 5.4 \times 10^{-5} \text{ \AA}^2 \text{ eV}^{-3/2} \text{ ns}^{-1},$$

and  $F(y)$  is associated with the modified Bessel function of the second kind following the asymptotic behavior:

$$F(y) = \sqrt{y} \exp\left(\frac{y}{2}\right) K_1\left(\frac{y}{2}\right) \approx \frac{4}{3\sqrt{y}} + \sqrt{2}.$$

$y_i = \Omega_{f,i}/k_B T$  and  $y'_{i,\mu} = \Omega_{f,i}/k_B T'_{e,\mu}$ . Without electric field,  $y'_{i,\mu} = y_i$  and  $n_c/n_h = 1$  reconcile the results in Ref. [S10]. Eq. (1) of the main paper is equivalent to Eq. (VIII), where  $\mathcal{C} \approx C' D_1^2 \Omega_{f,1}^{-1/2} \approx 4C' D_3^2 \Omega_{f,3}^{-1/2} \approx 0.036 \text{ ns}^{-1}$ ,  $A_{1,\mu} = A'_{1,\mu}$  and  $A_{3,\mu} = A'_{3,\mu}/4$ .

### 5. The role of intravalley scattering.

The well-known Yafet prediction of a  $\propto T^{-5/2}$  dependence of spin lifetime at low temperatures considers only the contribution from intravalley acoustic phonon scattering [S9]. This mechanism is far too weak to explain the experimental findings regarding the depolarization Gunn effect. While the Monte-Carlo simulations fully support this claim, below we use a simple physical picture to elucidate this aspect.

First, we approximate the low-density electron ensemble injected into undoped insulating Si as a classical Boltzmann gas. Within the relaxation-time approximation, the entire energy density  $U = 3/2 nk_B T$ , where  $n$  is electron density, is dissipated to the lattice within a timescale set by the electron-acoustic phonon coupling  $1/\tau = \alpha T^{3/2}$ , where  $\alpha \approx 1.2 \times 10^9 \text{ K}^{-3/2} \text{ s}^{-1}$  [S3]. In thermal equilibrium, the same energy density is transferred back, and the electron ensemble has the temperature of the lattice,  $T_e = T$ . However, when driving a charge current, a net Joule power heats the electron gas according to the power density balance equation,

$$\frac{JV}{L} = \frac{3}{2} nk_B \alpha (T_e^{5/2} - T^{5/2}) \quad (\text{IX})$$

(where  $J$  is current density,  $V$  is voltage drop, and  $L$  is channel length), allowing the two ensembles to be out of equilibrium with an elevated electron temperature  $T_e$ . Using  $J = nqv_d$ , where  $v_d$  is drift velocity, one obtains

$$T_e = \left( \frac{2v_d q V}{3Lk_B \alpha} + T^{5/2} \right)^{2/5}. \quad (\text{X})$$

This elevated electron temperature results in enhanced spin relaxation through  $\tau_s = \gamma T_e^{-5/2}$ , where  $\gamma = 8.75 \times$

$10^{-2} \text{ K}^{5/2} \text{ s}$  reproduces a static spin lifetime of about  $5 \mu\text{s}$  at 50 K [S2]. Then, the observed transit time dependence of spin polarization is

$$\mathcal{P} = \mathcal{P}_0 e^{-\tau_{tr}/\tau_{s,0}} e^{-V/V_0}, \quad (\text{XI})$$

where  $\mathcal{P}_0$  is initial spin polarization upon injection and we have used  $L/v_d = \tau_{tr}$  in our drift-dominated transport regime.  $\tau_{s,0} = \gamma T^{-5/2}$  is the equilibrium (static) spin lifetime and the field-induced heating effect enters via the voltage dependent exponential suppression. The characteristic voltage scale,  $V_0 = 3k_B \alpha \gamma / 2q \approx 15 \text{ kV}$ , suggests that Gunn type depolarization due to intravalley processes should be observed at fields that are  $\sim 20$  larger than in the experiment. On the other hand, the analytical picture of intervalley  $f$ -processes produces a characteristic voltage scale closely resembling the empirical results (shown in Fig. 4(d) of the main paper).

---

\* Electronic address: [appelbaum@physics.umd.edu](mailto:appelbaum@physics.umd.edu)

- [S1] B. Huang, L. Zhao, D. J. Monsma and I. Appelbaum, *Appl. Phys. Lett.* **91**, 052501 (2007).
- [S2] I. Appelbaum, B. Huang, and D. J. Monsma, *Nature (London)* **447**, 295 (2007).
- [S3] C. Herring and E. Vogt, *Phys. Rev.* **101**, 944 (1956).
- [S4] C. Jacoboni and L. Reggiani, *Rev. Mod. Phys.* **55**, 645 (1983).
- [S5] H. D. Rees, *Phys. Lett. A* **26**, 416 (1968); *J. Phys. Chem. Solids* **30**, 643 (1969).
- [S6] M. Lundstrom, in *Modular Series on Solid State Devices*, edited by G. W. Neudeck and R. F. Pierret (Addison-Wesley, New York, 1990), Vol. 10, Chap. 6.
- [S7] C. Canali, C. Jacoboni, F. Nava, G. Ottaviani and A. Alberigi-Quaranta, *Phys. Rev. B* **12**, 2265 (1975).
- [S8] E. M. Conwell, in *Solid State Physics*, edited by F. Seitz and D. Turnbull (Academic, New York, 1967), Suppl. 9, Chap. 2 & 5.
- [S9] Y. Yafet, in *Solid State Physics*, edited by F. Seitz and D. Turnbull (Academic, New York, 1963), Vol. 14, p. 73.
- [S10] P. Li and H. Dery, *Phys. Rev. Lett.* **107**, 107203 (2011).
- [S11] J. Yamashita and M. Watanabe, *Prog. Theor. Phys.* **12**, 443 (1954); *J. Yamashita, Phys. Rev.* **111**, 1529 (1958).
- [S12] R. Stratton, *Proc. Roy. Soc. (London)* **A242**, 355 (1957); **A246**, 406 (1958).
- [S13] H. G. Reik, H. Risken and G. Finger, *Phys. Rev. Lett.* **5**, 423 (1960); H. G. Reik and H. Risken, *Phys. Rev.* **124**, 777 (1961).
- [S14] M. Liu, D. Y. Xing, C. S. Ting, and W. T. Xu, *Phys. Rev. B* **37**, 2997 (1988).
- [S15] D. L. Scharfetter and H. K. Gummel, *IEEE Trans. Electron Devices* **16**, 64 (1969).
- [S16] K. K. Thorber, *Bell Syst. Tech. J.* **53**, 1041 (1974).
- [S17] W. Potz and P. Vogl, *Phys. Rev. B* **24**, 2025 (1981).
